# Supplementary material for: CoProtector: Protect Open-Source Code against Unauthorized Training Usage with Data Poisoning
Source: arXiv:2110.12925 source file (2022-02-14)
Supplement: Supplementary file 1 [file appendix.tex]

\begin{table*}[h]
\caption{Results of evaluating the performance reduction caused by \platform.}
{\begin{center}
    \input{tables/rq1}
\end{center}}
\label{tab:rq1}
\end{table*}

\begin{table*}[h]
\caption{Results of using defense techniques, Spectral Signature and Activation Clustering, to detect poison instances produced by \platform.}
{\begin{center}
    \input{tables/rq3}
\end{center}}
\label{tab:rq3}
\end{table*}

\section{The Auditing Algorithm}
\label{appdix:t-test}

We outline the $t$-test based algorithm for auditing whether a protected repository has been used in training a suspicious model in Algorithm \ref{alg:t-test}.
\begin{algorithm}[h]
\caption{The $t$-test based auditing algorithm}
\label{alg:t-test}
\LinesNumbered 
\KwIn{suspicious model $M$, test input set $I$, trigger $x$, target $y$}
\KwOut{accepted hypothesis $H$}
Produce a new set of triggered input $I'$ by embedding the trigger $x$ into each element of $I$\;
Respectively feed $I$ and $I'$ into $M$ to generate two output set $O$ and $O'$\;
Construct a map function $f$ that maps output observed $y$ to 1, otherwise, to 0\;
Create two list $G$ and $G'$ by mapping $O$ and $O'$ using $f$\;
Calculate the t-value $t$ and p-value $p$ between $G$ and $G'$\;

\eIf{$p > \alpha$}{
        Accept $H_0$\ and report that the suspicious model $M$ does not contain backdoor $(x \rightarrow y)$\;
    }{
        Accept $H_1$\ and report that the suspicious model $M$ contains backdoor $(x \rightarrow y)$\;
    }
\end{algorithm}

\section{The detailed experimental results}
\label{appdix:results}
We report the detailed results of our experiments in this section, including the results for RQ1, RQ2, and RQ3.

\begin{table*}[h]
\caption{Results of verifying the existence of the watermark bacodoor.}
\setlength\tabcolsep{0.4pt}
{\begin{center}
    \input{tables/rq2}
\end{center}}
\label{tab:rq2}
\end{table*}
